# Supplementary material for: AI-inferred expressed well-being and collective-action discourse in climate-change campaigns on X
Source: arXiv:2609.22096 source file (2026-08-11)
Supplement: Supplementary file 2 [file si_table_event_study_models.tex]

\begin{longtable}{llrrrrrrrrrrllll}
\caption{Segmented event-study and pretrend models.} \label{tab:event-study} \\
\toprule
model & term & estimate & estimate_pp & std_error & ci_low & ci_high & ci_low_pp & ci_high_pp & p_value & n & clusters & status & scope & component & reason \\
\midrule
\endfirsthead
\caption[]{Segmented event-study and pretrend models.} \\
\toprule
model & term & estimate & estimate_pp & std_error & ci_low & ci_high & ci_low_pp & ci_high_pp & p_value & n & clusters & status & scope & component & reason \\
\midrule
\endhead
\midrule
\multicolumn{16}{r}{Continued on next page} \\
\midrule
\endfoot
\bottomrule
\endlastfoot
all_campaigns_pretrend & Intercept & -9.210261 & -921.026095 & 6.057320 & -21.082389 & 2.661867 & -2108.238928 & 266.186739 & 0.128381 & 489 & 19.000000 & ok & all_campaigns & pretrend & NaN \\
all_campaigns_pretrend & C(day_of_week)[T.1] & 0.004775 & 0.477480 & 0.016562 & -0.027685 & 0.037235 & -2.768536 & 3.723495 & 0.773113 & 489 & 19.000000 & ok & all_campaigns & pretrend & NaN \\
all_campaigns_pretrend & C(day_of_week)[T.2] & -0.010130 & -1.012981 & 0.014138 & -0.037839 & 0.017580 & -3.783945 & 1.757983 & 0.473680 & 489 & 19.000000 & ok & all_campaigns & pretrend & NaN \\
all_campaigns_pretrend & C(day_of_week)[T.3] & 0.023544 & 2.354449 & 0.024339 & -0.024159 & 0.071248 & -2.415904 & 7.124801 & 0.333366 & 489 & 19.000000 & ok & all_campaigns & pretrend & NaN \\
all_campaigns_pretrend & C(day_of_week)[T.4] & 0.006329 & 0.632940 & 0.012648 & -0.018460 & 0.031119 & -1.846041 & 3.111922 & 0.616777 & 489 & 19.000000 & ok & all_campaigns & pretrend & NaN \\
all_campaigns_pretrend & C(day_of_week)[T.5] & 0.001039 & 0.103898 & 0.016915 & -0.032115 & 0.034193 & -3.211476 & 3.419272 & 0.951023 & 489 & 19.000000 & ok & all_campaigns & pretrend & NaN \\
all_campaigns_pretrend & C(day_of_week)[T.6] & 0.000366 & 0.036607 & 0.018847 & -0.036573 & 0.037305 & -3.657330 & 3.730543 & 0.984504 & 489 & 19.000000 & ok & all_campaigns & pretrend & NaN \\
all_campaigns_pretrend & days_from_event & -0.000186 & -0.018634 & 0.000971 & -0.002090 & 0.001717 & -0.208971 & 0.171703 & 0.847838 & 489 & 19.000000 & ok & all_campaigns & pretrend & NaN \\
all_campaigns_pretrend & log_n_tweets & -0.002577 & -0.257717 & 0.007997 & -0.018251 & 0.013096 & -1.825068 & 1.309634 & 0.747245 & 489 & 19.000000 & ok & all_campaigns & pretrend & NaN \\
all_campaigns_pretrend & event_year & 0.004589 & 0.458882 & 0.003001 & -0.001293 & 0.010471 & -0.129301 & 1.047065 & 0.126239 & 489 & 19.000000 & ok & all_campaigns & pretrend & NaN \\
all_campaigns_segmented_event_study & Intercept & -2.653269 & -265.326893 & 7.999294 & -18.331598 & 13.025060 & -1833.159780 & 1302.505994 & 0.740125 & 1008 & 19.000000 & ok & all_campaigns & segmented_event_study & NaN \\
all_campaigns_segmented_event_study & C(period)[T.event] & 0.054092 & 5.409167 & 0.028314 & -0.001402 & 0.109585 & -0.140181 & 10.958515 & 0.056075 & 1008 & 19.000000 & ok & all_campaigns & segmented_event_study & NaN \\
all_campaigns_segmented_event_study & C(period)[T.post] & 0.018944 & 1.894375 & 0.028573 & -0.037059 & 0.074947 & -3.705904 & 7.494654 & 0.507340 & 1008 & 19.000000 & ok & all_campaigns & segmented_event_study & NaN \\
all_campaigns_segmented_event_study & C(day_of_week)[T.1] & 0.010102 & 1.010154 & 0.014489 & -0.018296 & 0.038499 & -1.829565 & 3.849874 & 0.485675 & 1008 & 19.000000 & ok & all_campaigns & segmented_event_study & NaN \\
all_campaigns_segmented_event_study & C(day_of_week)[T.2] & -0.002731 & -0.273056 & 0.011543 & -0.025355 & 0.019894 & -2.535522 & 1.989410 & 0.813008 & 1008 & 19.000000 & ok & all_campaigns & segmented_event_study & NaN \\
all_campaigns_segmented_event_study & C(day_of_week)[T.3] & 0.006779 & 0.677947 & 0.013737 & -0.020145 & 0.033704 & -2.014502 & 3.370395 & 0.621652 & 1008 & 19.000000 & ok & all_campaigns & segmented_event_study & NaN \\
all_campaigns_segmented_event_study & C(day_of_week)[T.4] & 0.002415 & 0.241474 & 0.012539 & -0.022161 & 0.026990 & -2.216057 & 2.699005 & 0.847285 & 1008 & 19.000000 & ok & all_campaigns & segmented_event_study & NaN \\
all_campaigns_segmented_event_study & C(day_of_week)[T.5] & 0.005253 & 0.525286 & 0.015979 & -0.026065 & 0.036571 & -2.606518 & 3.657090 & 0.742354 & 1008 & 19.000000 & ok & all_campaigns & segmented_event_study & NaN \\
all_campaigns_segmented_event_study & C(day_of_week)[T.6] & -0.001476 & -0.147577 & 0.010888 & -0.022816 & 0.019864 & -2.281555 & 1.986402 & 0.892183 & 1008 & 19.000000 & ok & all_campaigns & segmented_event_study & NaN \\
all_campaigns_segmented_event_study & days_from_event & 0.000132 & 0.013210 & 0.000711 & -0.001261 & 0.001525 & -0.126097 & 0.152517 & 0.852558 & 1008 & 19.000000 & ok & all_campaigns & segmented_event_study & NaN \\
all_campaigns_segmented_event_study & days_from_event:C(period)[T.event] & -0.000000 & -0.000000 & 0.000000 & -0.000000 & 0.000000 & -0.000000 & 0.000000 & 0.748700 & 1008 & 19.000000 & ok & all_campaigns & segmented_event_study & NaN \\
all_campaigns_segmented_event_study & days_from_event:C(period)[T.post] & -0.001191 & -0.119058 & 0.001452 & -0.004036 & 0.001655 & -0.403570 & 0.165454 & 0.412116 & 1008 & 19.000000 & ok & all_campaigns & segmented_event_study & NaN \\
all_campaigns_segmented_event_study & log_n_tweets & -0.005706 & -0.570555 & 0.004571 & -0.014665 & 0.003254 & -1.466522 & 0.325412 & 0.211990 & 1008 & 19.000000 & ok & all_campaigns & segmented_event_study & NaN \\
all_campaigns_segmented_event_study & event_year & 0.001347 & 0.134725 & 0.003963 & -0.006419 & 0.009114 & -0.641936 & 0.911387 & 0.733864 & 1008 & 19.000000 & ok & all_campaigns & segmented_event_study & NaN \\
earth_day_pretrend & Intercept & -20.056508 & -2005.650815 & 9.272986 & -38.231227 & -1.881789 & -3823.122689 & -188.178941 & 0.030549 & 224 & 8.000000 & ok & earth_day & pretrend & NaN \\
earth_day_pretrend & C(day_of_week)[T.1] & -0.021842 & -2.184217 & 0.028838 & -0.078364 & 0.034680 & -7.836439 & 3.468005 & 0.448811 & 224 & 8.000000 & ok & earth_day & pretrend & NaN \\
earth_day_pretrend & C(day_of_week)[T.2] & -0.038451 & -3.845141 & 0.026600 & -0.090586 & 0.013683 & -9.058595 & 1.368314 & 0.148302 & 224 & 8.000000 & ok & earth_day & pretrend & NaN \\
earth_day_pretrend & C(day_of_week)[T.3] & -0.029414 & -2.941392 & 0.013336 & -0.055552 & -0.003275 & -5.555247 & -0.327537 & 0.027415 & 224 & 8.000000 & ok & earth_day & pretrend & NaN \\
earth_day_pretrend & C(day_of_week)[T.4] & -0.004750 & -0.475025 & 0.018724 & -0.041449 & 0.031948 & -4.144868 & 3.194818 & 0.799729 & 224 & 8.000000 & ok & earth_day & pretrend & NaN \\
earth_day_pretrend & C(day_of_week)[T.5] & -0.024207 & -2.420719 & 0.024369 & -0.071970 & 0.023556 & -7.196995 & 2.355557 & 0.320539 & 224 & 8.000000 & ok & earth_day & pretrend & NaN \\
earth_day_pretrend & C(day_of_week)[T.6] & -0.004146 & -0.414640 & 0.038765 & -0.080124 & 0.071831 & -8.012403 & 7.183123 & 0.914818 & 224 & 8.000000 & ok & earth_day & pretrend & NaN \\
earth_day_pretrend & days_from_event & -0.002389 & -0.238937 & 0.001864 & -0.006044 & 0.001265 & -0.604366 & 0.126492 & 0.200008 & 224 & 8.000000 & ok & earth_day & pretrend & NaN \\
earth_day_pretrend & log_n_tweets & 0.007530 & 0.753001 & 0.009605 & -0.011296 & 0.026356 & -1.129627 & 2.635630 & 0.433079 & 224 & 8.000000 & ok & earth_day & pretrend & NaN \\
earth_day_pretrend & event_year & 0.009955 & 0.995509 & 0.004604 & 0.000932 & 0.018978 & 0.093194 & 1.897824 & 0.030588 & 224 & 8.000000 & ok & earth_day & pretrend & NaN \\
earth_day_segmented_event_study & Intercept & -3.614459 & -361.445948 & 10.490264 & -24.175000 & 16.946081 & -2417.499971 & 1694.608075 & 0.730430 & 469 & 8.000000 & ok & earth_day & segmented_event_study & NaN \\
earth_day_segmented_event_study & C(period)[T.event] & 0.130033 & 13.003327 & 0.066155 & 0.000372 & 0.259695 & 0.037167 & 25.969487 & 0.049347 & 469 & 8.000000 & ok & earth_day & segmented_event_study & NaN \\
earth_day_segmented_event_study & C(period)[T.post] & 0.044868 & 4.486833 & 0.064981 & -0.082492 & 0.172229 & -8.249217 & 17.222882 & 0.489890 & 469 & 8.000000 & ok & earth_day & segmented_event_study & NaN \\
earth_day_segmented_event_study & C(day_of_week)[T.1] & 0.018907 & 1.890704 & 0.027549 & -0.035087 & 0.072901 & -3.508712 & 7.290121 & 0.492513 & 469 & 8.000000 & ok & earth_day & segmented_event_study & NaN \\
earth_day_segmented_event_study & C(day_of_week)[T.2] & -0.000661 & -0.066095 & 0.021196 & -0.042203 & 0.040882 & -4.220346 & 4.088156 & 0.975123 & 469 & 8.000000 & ok & earth_day & segmented_event_study & NaN \\
earth_day_segmented_event_study & C(day_of_week)[T.3] & -0.001052 & -0.105186 & 0.007277 & -0.015315 & 0.013212 & -1.531528 & 1.321156 & 0.885076 & 469 & 8.000000 & ok & earth_day & segmented_event_study & NaN \\
earth_day_segmented_event_study & C(day_of_week)[T.4] & 0.005653 & 0.565269 & 0.014237 & -0.022252 & 0.033557 & -2.225172 & 3.355709 & 0.691341 & 469 & 8.000000 & ok & earth_day & segmented_event_study & NaN \\
earth_day_segmented_event_study & C(day_of_week)[T.5] & 0.016201 & 1.620131 & 0.027512 & -0.037720 & 0.070123 & -3.772050 & 7.012311 & 0.555935 & 469 & 8.000000 & ok & earth_day & segmented_event_study & NaN \\
earth_day_segmented_event_study & C(day_of_week)[T.6] & 0.009204 & 0.920387 & 0.017534 & -0.025163 & 0.043570 & -2.516259 & 4.357033 & 0.599647 & 469 & 8.000000 & ok & earth_day & segmented_event_study & NaN \\
earth_day_segmented_event_study & days_from_event & 0.000989 & 0.098936 & 0.001632 & -0.002210 & 0.004188 & -0.220978 & 0.418850 & 0.544426 & 469 & 8.000000 & ok & earth_day & segmented_event_study & NaN \\
earth_day_segmented_event_study & days_from_event:C(period)[T.event] & -0.000000 & -0.000000 & 0.000000 & -0.000000 & 0.000000 & -0.000000 & 0.000000 & 0.691341 & 469 & 8.000000 & ok & earth_day & segmented_event_study & NaN \\
earth_day_segmented_event_study & days_from_event:C(period)[T.post] & -0.004215 & -0.421465 & 0.004074 & -0.012200 & 0.003771 & -1.219990 & 0.377060 & 0.300913 & 469 & 8.000000 & ok & earth_day & segmented_event_study & NaN \\
earth_day_segmented_event_study & log_n_tweets & -0.015118 & -1.511787 & 0.009587 & -0.033909 & 0.003673 & -3.390888 & 0.367314 & 0.114832 & 469 & 8.000000 & ok & earth_day & segmented_event_study & NaN \\
earth_day_segmented_event_study & event_year & 0.001856 & 0.185633 & 0.005192 & -0.008319 & 0.012032 & -0.831913 & 1.203178 & 0.720673 & 469 & 8.000000 & ok & earth_day & segmented_event_study & NaN \\
earth_hour_pretrend & Intercept & -0.024343 & -2.434268 & 5.597353 & -10.994952 & 10.946267 & -1099.495224 & 1094.626688 & 0.996530 & 99 & 4.000000 & ok & earth_hour & pretrend & NaN \\
earth_hour_pretrend & C(day_of_week)[T.1] & 0.006712 & 0.671230 & 0.028832 & -0.049797 & 0.063222 & -4.979711 & 6.322171 & 0.815910 & 99 & 4.000000 & ok & earth_hour & pretrend & NaN \\
earth_hour_pretrend & C(day_of_week)[T.2] & -0.012315 & -1.231459 & 0.009527 & -0.030987 & 0.006358 & -3.098739 & 0.635822 & 0.196156 & 99 & 4.000000 & ok & earth_hour & pretrend & NaN \\
earth_hour_pretrend & C(day_of_week)[T.3] & 0.046430 & 4.643010 & 0.047186 & -0.046053 & 0.138913 & -4.605310 & 13.891331 & 0.325127 & 99 & 4.000000 & ok & earth_hour & pretrend & NaN \\
earth_hour_pretrend & C(day_of_week)[T.4] & -0.006946 & -0.694635 & 0.019131 & -0.044442 & 0.030550 & -4.444239 & 3.054968 & 0.716534 & 99 & 4.000000 & ok & earth_hour & pretrend & NaN \\
earth_hour_pretrend & C(day_of_week)[T.5] & -0.019909 & -1.990889 & 0.011634 & -0.042711 & 0.002894 & -4.271140 & 0.289361 & 0.087036 & 99 & 4.000000 & ok & earth_hour & pretrend & NaN \\
earth_hour_pretrend & C(day_of_week)[T.6] & -0.001644 & -0.164421 & 0.006858 & -0.015086 & 0.011798 & -1.508594 & 1.179752 & 0.810528 & 99 & 4.000000 & ok & earth_hour & pretrend & NaN \\
earth_hour_pretrend & days_from_event & 0.000537 & 0.053734 & 0.000613 & -0.000665 & 0.001740 & -0.066508 & 0.173975 & 0.381102 & 99 & 4.000000 & ok & earth_hour & pretrend & NaN \\
earth_hour_pretrend & log_n_tweets & -0.004830 & -0.483003 & 0.003244 & -0.011189 & 0.001529 & -1.118910 & 0.152904 & 0.136569 & 99 & 4.000000 & ok & earth_hour & pretrend & NaN \\
earth_hour_pretrend & event_year & 0.000033 & 0.003281 & 0.002779 & -0.005414 & 0.005480 & -0.541423 & 0.547984 & 0.990582 & 99 & 4.000000 & ok & earth_hour & pretrend & NaN \\
earth_hour_segmented_event_study & Intercept & 0.126742 & 12.674157 & 4.870963 & -9.420170 & 9.673654 & -942.017047 & 967.365362 & 0.979242 & 194 & 4.000000 & ok & earth_hour & segmented_event_study & NaN \\
earth_hour_segmented_event_study & C(period)[T.event] & -0.010993 & -1.099290 & 0.015590 & -0.041549 & 0.019563 & -4.154879 & 1.956299 & 0.480733 & 194 & 4.000000 & ok & earth_hour & segmented_event_study & NaN \\
earth_hour_segmented_event_study & C(period)[T.post] & 0.003051 & 0.305050 & 0.023817 & -0.043630 & 0.049731 & -4.362983 & 4.973084 & 0.898085 & 194 & 4.000000 & ok & earth_hour & segmented_event_study & NaN \\
earth_hour_segmented_event_study & C(day_of_week)[T.1] & 0.003439 & 0.343949 & 0.030075 & -0.055507 & 0.062386 & -5.550667 & 6.238564 & 0.908950 & 194 & 4.000000 & ok & earth_hour & segmented_event_study & NaN \\
earth_hour_segmented_event_study & C(day_of_week)[T.2] & -0.008651 & -0.865110 & 0.023081 & -0.053888 & 0.036586 & -5.388833 & 3.658613 & 0.707794 & 194 & 4.000000 & ok & earth_hour & segmented_event_study & NaN \\
earth_hour_segmented_event_study & C(day_of_week)[T.3] & 0.019563 & 1.956320 & 0.029280 & -0.037824 & 0.076950 & -3.782367 & 7.695007 & 0.504036 & 194 & 4.000000 & ok & earth_hour & segmented_event_study & NaN \\
earth_hour_segmented_event_study & C(day_of_week)[T.4] & -0.005305 & -0.530495 & 0.012186 & -0.029190 & 0.018580 & -2.918975 & 1.857985 & 0.663331 & 194 & 4.000000 & ok & earth_hour & segmented_event_study & NaN \\
earth_hour_segmented_event_study & C(day_of_week)[T.5] & 0.008483 & 0.848347 & 0.022973 & -0.036543 & 0.053510 & -3.654266 & 5.350960 & 0.711918 & 194 & 4.000000 & ok & earth_hour & segmented_event_study & NaN \\
earth_hour_segmented_event_study & C(day_of_week)[T.6] & -0.009512 & -0.951194 & 0.012051 & -0.033131 & 0.014107 & -3.313070 & 1.410682 & 0.429917 & 194 & 4.000000 & ok & earth_hour & segmented_event_study & NaN \\
earth_hour_segmented_event_study & days_from_event & 0.000139 & 0.013861 & 0.000803 & -0.001435 & 0.001712 & -0.143482 & 0.171204 & 0.862919 & 194 & 4.000000 & ok & earth_hour & segmented_event_study & NaN \\
earth_hour_segmented_event_study & days_from_event:C(period)[T.event] & 0.000000 & 0.000000 & 0.000000 & -0.000000 & 0.000000 & -0.000000 & 0.000000 & 0.975705 & 194 & 4.000000 & ok & earth_hour & segmented_event_study & NaN \\
earth_hour_segmented_event_study & days_from_event:C(period)[T.post] & -0.000510 & -0.050952 & 0.002582 & -0.005570 & 0.004551 & -0.557024 & 0.455120 & 0.843568 & 194 & 4.000000 & ok & earth_hour & segmented_event_study & NaN \\
earth_hour_segmented_event_study & log_n_tweets & -0.000260 & -0.026005 & 0.001765 & -0.003720 & 0.003200 & -0.372010 & 0.319999 & 0.882888 & 194 & 4.000000 & ok & earth_hour & segmented_event_study & NaN \\
earth_hour_segmented_event_study & event_year & -0.000052 & -0.005156 & 0.002406 & -0.004768 & 0.004665 & -0.476790 & 0.466479 & 0.982906 & 194 & 4.000000 & ok & earth_hour & segmented_event_study & NaN \\
global_climate_action_day_pretrend & NaN & NaN & NaN & NaN & NaN & NaN & NaN & NaN & NaN & 30 & NaN & failed & global_climate_action_day & pretrend & float division by zero \\
global_climate_action_day_segmented_event_study & NaN & NaN & NaN & NaN & NaN & NaN & NaN & NaN & NaN & 61 & NaN & failed & global_climate_action_day & segmented_event_study & float division by zero \\
world_environment_day_pretrend & Intercept & -0.131071 & -13.107076 & 11.128840 & -21.943196 & 21.681054 & -2194.319603 & 2168.105450 & 0.990603 & 136 & 6.000000 & ok & world_environment_day & pretrend & NaN \\
world_environment_day_pretrend & C(day_of_week)[T.1] & 0.027384 & 2.738399 & 0.032301 & -0.035925 & 0.090693 & -3.592472 & 9.069269 & 0.396562 & 136 & 6.000000 & ok & world_environment_day & pretrend & NaN \\
world_environment_day_pretrend & C(day_of_week)[T.2] & 0.016007 & 1.600653 & 0.023542 & -0.030135 & 0.062148 & -3.013532 & 6.214839 & 0.496563 & 136 & 6.000000 & ok & world_environment_day & pretrend & NaN \\
world_environment_day_pretrend & C(day_of_week)[T.3] & 0.088540 & 8.853973 & 0.058568 & -0.026251 & 0.203331 & -2.625105 & 20.333051 & 0.130598 & 136 & 6.000000 & ok & world_environment_day & pretrend & NaN \\
world_environment_day_pretrend & C(day_of_week)[T.4] & 0.029413 & 2.941332 & 0.019478 & -0.008764 & 0.067590 & -0.876383 & 6.759047 & 0.131033 & 136 & 6.000000 & ok & world_environment_day & pretrend & NaN \\
world_environment_day_pretrend & C(day_of_week)[T.5] & 0.045538 & 4.553778 & 0.039710 & -0.032293 & 0.123368 & -3.229278 & 12.336834 & 0.251484 & 136 & 6.000000 & ok & world_environment_day & pretrend & NaN \\
world_environment_day_pretrend & C(day_of_week)[T.6] & -0.006993 & -0.699329 & 0.004821 & -0.016442 & 0.002456 & -1.644225 & 0.245567 & 0.146893 & 136 & 6.000000 & ok & world_environment_day & pretrend & NaN \\
world_environment_day_pretrend & days_from_event & 0.001300 & 0.130001 & 0.000464 & 0.000391 & 0.002209 & 0.039091 & 0.220912 & 0.005067 & 136 & 6.000000 & ok & world_environment_day & pretrend & NaN \\
world_environment_day_pretrend & log_n_tweets & -0.010387 & -1.038739 & 0.015900 & -0.041551 & 0.020776 & -4.155088 & 2.077609 & 0.513567 & 136 & 6.000000 & ok & world_environment_day & pretrend & NaN \\
world_environment_day_pretrend & event_year & 0.000088 & 0.008822 & 0.005511 & -0.010713 & 0.010889 & -1.071300 & 1.088945 & 0.987228 & 136 & 6.000000 & ok & world_environment_day & pretrend & NaN \\
world_environment_day_segmented_event_study & Intercept & -7.978337 & -797.833663 & 4.256832 & -16.321574 & 0.364901 & -1632.157417 & 36.490092 & 0.060897 & 284 & 6.000000 & ok & world_environment_day & segmented_event_study & NaN \\
world_environment_day_segmented_event_study & C(period)[T.event] & 0.072258 & 7.225768 & 0.022520 & 0.028119 & 0.116396 & 2.811895 & 11.639641 & 0.001334 & 284 & 6.000000 & ok & world_environment_day & segmented_event_study & NaN \\
world_environment_day_segmented_event_study & C(period)[T.post] & 0.030768 & 3.076807 & 0.031054 & -0.030097 & 0.091633 & -3.009705 & 9.163320 & 0.321790 & 284 & 6.000000 & ok & world_environment_day & segmented_event_study & NaN \\
world_environment_day_segmented_event_study & C(day_of_week)[T.1] & 0.007701 & 0.770053 & 0.033063 & -0.057101 & 0.072502 & -5.710109 & 7.250215 & 0.815834 & 284 & 6.000000 & ok & world_environment_day & segmented_event_study & NaN \\
world_environment_day_segmented_event_study & C(day_of_week)[T.2] & 0.003103 & 0.310332 & 0.030368 & -0.056416 & 0.062623 & -5.641650 & 6.262313 & 0.918605 & 284 & 6.000000 & ok & world_environment_day & segmented_event_study & NaN \\
world_environment_day_segmented_event_study & C(day_of_week)[T.3] & 0.016831 & 1.683085 & 0.043466 & -0.068360 & 0.102022 & -6.836046 & 10.202216 & 0.698593 & 284 & 6.000000 & ok & world_environment_day & segmented_event_study & NaN \\
world_environment_day_segmented_event_study & C(day_of_week)[T.4] & 0.009223 & 0.922316 & 0.039840 & -0.068861 & 0.087307 & -6.886095 & 8.730728 & 0.816920 & 284 & 6.000000 & ok & world_environment_day & segmented_event_study & NaN \\
world_environment_day_segmented_event_study & C(day_of_week)[T.5] & -0.008306 & -0.830642 & 0.036638 & -0.080116 & 0.063503 & -8.011632 & 6.350347 & 0.820646 & 284 & 6.000000 & ok & world_environment_day & segmented_event_study & NaN \\
world_environment_day_segmented_event_study & C(day_of_week)[T.6] & -0.019392 & -1.939188 & 0.027523 & -0.073337 & 0.034553 & -7.333680 & 3.455305 & 0.481085 & 284 & 6.000000 & ok & world_environment_day & segmented_event_study & NaN \\
world_environment_day_segmented_event_study & days_from_event & 0.001254 & 0.125425 & 0.000836 & -0.000384 & 0.002893 & -0.038419 & 0.289270 & 0.133515 & 284 & 6.000000 & ok & world_environment_day & segmented_event_study & NaN \\
world_environment_day_segmented_event_study & days_from_event:C(period)[T.event] & 0.000000 & 0.000000 & 0.000000 & -0.000000 & 0.000000 & -0.000000 & 0.000000 & 0.131049 & 284 & 6.000000 & ok & world_environment_day & segmented_event_study & NaN \\
world_environment_day_segmented_event_study & days_from_event:C(period)[T.post] & -0.003913 & -0.391297 & 0.001545 & -0.006942 & -0.000884 & -0.694185 & -0.088408 & 0.011340 & 284 & 6.000000 & ok & world_environment_day & segmented_event_study & NaN \\
world_environment_day_segmented_event_study & log_n_tweets & -0.012901 & -1.290146 & 0.007321 & -0.027251 & 0.001448 & -2.725116 & 0.144823 & 0.078043 & 284 & 6.000000 & ok & world_environment_day & segmented_event_study & NaN \\
world_environment_day_segmented_event_study & event_year & 0.003991 & 0.399143 & 0.002101 & -0.000127 & 0.008110 & -0.012724 & 0.811009 & 0.057510 & 284 & 6.000000 & ok & world_environment_day & segmented_event_study & NaN \\
\end{longtable}
