# Supplementary material for: AI-inferred expressed well-being and collective-action discourse in climate-change campaigns on X
Source: arXiv:2609.22096 source file (2026-08-11)
Supplement: Supplementary file 3 [file si_table_external_validation_summary.tex]

\begin{longtable}{llrrrrrlll}
\caption{External dictionary controls for the learned expressed-well-being scores.} \label{tab:external-validation} \\
\toprule
pair & scope & n\_cells & pearson\_r & pearson\_p & spearman\_rho & spearman\_p & validation\_family & liwc\_metric & ai\_metric \\
\midrule
\endfirsthead
\caption[]{External dictionary controls for the learned expressed-well-being scores.} \\
\toprule
pair & scope & n\_cells & pearson\_r & pearson\_p & spearman\_rho & spearman\_p & validation\_family & liwc\_metric & ai\_metric \\
\midrule
\endhead
\midrule
\multicolumn{10}{r}{Continued on next page} \\
\midrule
\endfoot
\bottomrule
\endlastfoot
labMT happiness mean vs AI happiness prevalence & all periods & 57 & 0.337881 & 0.010155 & 0.199831 & 0.136133 & labMT & NaN & NaN \\
labMT positive-word share vs AI happiness prevalence & all periods & 57 & 0.354160 & 0.006875 & 0.372764 & 0.004295 & labMT & NaN & NaN \\
NaN & all periods & 57 & 0.550314 & 0.000009 & 0.561382 & 0.000006 & LIWC2007 & liwc\_posemo\_prop & ai\_happiness\_mean \\
NaN & all periods & 57 & 0.564899 & 0.000005 & 0.578299 & 0.000002 & LIWC2007 & liwc\_posemo\_prop & ai\_happiness\_prevalence \\
NaN & all periods & 57 & 0.083541 & 0.536689 & 0.203011 & 0.129883 & LIWC2007 & liwc\_negemo\_prop & ai\_distress\_mean \\
NaN & all periods & 57 & 0.077702 & 0.565622 & 0.207993 & 0.120530 & LIWC2007 & liwc\_negemo\_prop & ai\_distress\_prevalence \\
NaN & all periods & 57 & -0.104817 & 0.437771 & 0.094817 & 0.482946 & LIWC2007 & liwc\_future\_prop & ai\_hope\_willpower\_mean \\
NaN & all periods & 57 & -0.098134 & 0.467694 & 0.100524 & 0.456870 & LIWC2007 & liwc\_future\_prop & ai\_hope\_willpower\_prevalence \\
NaN & all periods & 57 & 0.090780 & 0.501851 & 0.230814 & 0.084094 & LIWC2007 & liwc\_achieve\_prop & ai\_hope\_waypower\_mean \\
NaN & all periods & 57 & 0.213609 & 0.110609 & 0.334586 & 0.010963 & LIWC2007 & liwc\_achieve\_prop & ai\_hope\_waypower\_prevalence \\
NaN & all periods & 57 & 0.371964 & 0.004385 & 0.470419 & 0.000222 & LIWC2007 & liwc\_social\_prop & ai\_collective\_capability\_mean \\
NaN & all periods & 57 & 0.356499 & 0.006490 & 0.480401 & 0.000156 & LIWC2007 & liwc\_social\_prop & ai\_collective\_capability\_prevalence \\
NaN & all periods & 57 & -0.391197 & 0.002622 & -0.342300 & 0.009153 & LIWC2007 & liwc\_work\_prop & ai\_action\_mean \\
NaN & all periods & 57 & -0.377893 & 0.003754 & -0.329855 & 0.012220 & LIWC2007 & liwc\_work\_prop & ai\_action\_prevalence \\
\end{longtable}
