# Supplementary material for: AI-inferred expressed well-being and collective-action discourse in climate-change campaigns on X
Source: arXiv:2609.22096 source file (2026-08-11)
Supplement: Supplementary file 4 [file si_table_retweet_cascade_models.tex]

\begin{longtable}{llrrrrrrrrrrl}
\caption{Source happiness and observed retweet cascade size.} \label{tab:retweet-cascade} \\
\toprule
model & term & estimate & estimate_pp & std_error & ci_low & ci_high & ci_low_pp & ci_high_pp & p_value & n & clusters & status \\
\midrule
\endfirsthead
\caption[]{Source happiness and observed retweet cascade size.} \\
\toprule
model & term & estimate & estimate_pp & std_error & ci_low & ci_high & ci_low_pp & ci_high_pp & p_value & n & clusters & status \\
\midrule
\endhead
\midrule
\multicolumn{13}{r}{Continued on next page} \\
\midrule
\endfoot
\bottomrule
\endlastfoot
cascade_score_ols & Intercept & -0.096451 & -9.645099 & 0.067899 & -0.229532 & 0.036630 & -22.953153 & 3.662955 & 0.155463 & 7864 & 15 & ok \\
cascade_score_ols & C(period)[T.event] & -0.104705 & -10.470496 & 0.022651 & -0.149099 & -0.060311 & -14.909923 & -6.031068 & 0.000004 & 7864 & 15 & ok \\
cascade_score_ols & C(period)[T.post] & -0.063660 & -6.366021 & 0.025384 & -0.113413 & -0.013908 & -11.341291 & -1.390752 & 0.012147 & 7864 & 15 & ok \\
cascade_score_ols & C(campaign_family)[T.earth_hour] & -0.075214 & -7.521446 & 0.017788 & -0.110079 & -0.040350 & -11.007871 & -4.035022 & 0.000024 & 7864 & 15 & ok \\
cascade_score_ols & C(campaign_family)[T.global_climate_action_day] & 0.107218 & 10.721847 & 0.020575 & 0.066893 & 0.147544 & 6.689274 & 14.754420 & 0.000000 & 7864 & 15 & ok \\
cascade_score_ols & C(campaign_family)[T.world_environment_day] & 0.001245 & 0.124529 & 0.041566 & -0.080222 & 0.082712 & -8.022177 & 8.271235 & 0.976099 & 7864 & 15 & ok \\
cascade_score_ols & verified[T.True] & 0.054104 & 5.410429 & 0.026675 & 0.001822 & 0.106387 & 0.182185 & 10.638673 & 0.042534 & 7864 & 15 & ok \\
cascade_score_ols & source_happiness_score & -1.400247 & -140.024676 & 0.749948 & -2.870118 & 0.069624 & -287.011753 & 6.962401 & 0.061884 & 7864 & 15 & ok \\
cascade_score_ols & source_happiness_score:C(period)[T.event] & 1.554591 & 155.459140 & 0.519579 & 0.536235 & 2.572948 & 53.623472 & 257.294808 & 0.002771 & 7864 & 15 & ok \\
cascade_score_ols & source_happiness_score:C(period)[T.post] & 1.252455 & 125.245516 & 0.547939 & 0.178514 & 2.326396 & 17.851384 & 232.639648 & 0.022269 & 7864 & 15 & ok \\
cascade_score_ols & log_followers & 0.170649 & 17.064929 & 0.006672 & 0.157572 & 0.183726 & 15.757210 & 18.372649 & 0.000000 & 7864 & 15 & ok \\
cascade_presence_ols & Intercept & -0.100313 & -10.031283 & 0.067568 & -0.232744 & 0.032118 & -23.274358 & 3.211791 & 0.137644 & 7864 & 15 & ok \\
cascade_presence_ols & C(period)[T.event] & -0.103887 & -10.388674 & 0.023125 & -0.149212 & -0.058562 & -14.921155 & -5.856194 & 0.000007 & 7864 & 15 & ok \\
cascade_presence_ols & C(period)[T.post] & -0.065466 & -6.546602 & 0.025402 & -0.115254 & -0.015678 & -11.525371 & -1.567832 & 0.009961 & 7864 & 15 & ok \\
cascade_presence_ols & C(campaign_family)[T.earth_hour] & -0.073007 & -7.300700 & 0.017417 & -0.107143 & -0.038871 & -10.714329 & -3.887071 & 0.000028 & 7864 & 15 & ok \\
cascade_presence_ols & C(campaign_family)[T.global_climate_action_day] & 0.109775 & 10.977529 & 0.020630 & 0.069341 & 0.150209 & 6.934114 & 15.020945 & 0.000000 & 7864 & 15 & ok \\
cascade_presence_ols & C(campaign_family)[T.world_environment_day] & 0.002558 & 0.255828 & 0.041335 & -0.078457 & 0.083574 & -7.845741 & 8.357397 & 0.950650 & 7864 & 15 & ok \\
cascade_presence_ols & verified[T.True] & 0.053727 & 5.372696 & 0.026741 & 0.001315 & 0.106139 & 0.131482 & 10.613909 & 0.044523 & 7864 & 15 & ok \\
cascade_presence_ols & source_happiness_presence & -0.130113 & -13.011323 & 0.079057 & -0.285062 & 0.024836 & -28.506212 & 2.483567 & 0.099802 & 7864 & 15 & ok \\
cascade_presence_ols & source_happiness_presence:C(period)[T.event] & 0.161175 & 16.117525 & 0.051526 & 0.060186 & 0.262164 & 6.018625 & 26.216425 & 0.001760 & 7864 & 15 & ok \\
cascade_presence_ols & source_happiness_presence:C(period)[T.post] & 0.134329 & 13.432875 & 0.051776 & 0.032850 & 0.235807 & 3.285028 & 23.580722 & 0.009475 & 7864 & 15 & ok \\
cascade_presence_ols & log_followers & 0.170867 & 17.086672 & 0.006697 & 0.157740 & 0.183993 & 15.774043 & 18.399301 & 0.000000 & 7864 & 15 & ok \\
\end{longtable}
