# Supplementary material for: AI-inferred expressed well-being and collective-action discourse in climate-change campaigns on X
Source: arXiv:2609.22096 source file (2026-08-11)
Supplement: Supplementary file 5 [file si_table_table_H1_happiness_temporal.tex]

\begin{longtable}{llllllllll}
\caption{Human-only happiness changes across campaign periods.}\label{tab:happiness-temporal}\\
\toprule
measure & measure\_label & contrast & n\_occurrence\_years & mean\_difference & ci\_low & ci\_high & wilcoxon\_statistic & p\_value & q\_value\_bh \\
\midrule
\endfirsthead
\toprule
measure & measure\_label & contrast & n\_occurrence\_years & mean\_difference & ci\_low & ci\_high & wilcoxon\_statistic & p\_value & q\_value\_bh \\
\midrule
\endhead
happiness\_prevalence & Happiness prevalence & event\_minus\_pre & 19 & 0.04944 & 0.02033 & 0.07856 & 19 & 0.001171 & 0.001561 \\
happiness\_prevalence & Happiness prevalence & post\_minus\_pre & 19 & 0.03392 & 0.008263 & 0.05958 & 38 & 0.02041 & 0.02041 \\
happiness\_mean & Happiness score & event\_minus\_pre & 19 & 0.01301 & 0.004942 & 0.02109 & 7 & 7.248e-05 & 0.0002899 \\
happiness\_mean & Happiness score & post\_minus\_pre & 19 & 0.009266 & 0.002948 & 0.01558 & 16 & 0.0006447 & 0.001289 \\
\bottomrule
\end{longtable}
