# Supplementary material for: AI-inferred expressed well-being and collective-action discourse in climate-change campaigns on X
Source: arXiv:2609.22096 source file (2026-08-11)
Supplement: Supplementary file 6 [file si_table_table_RQ3_direct_decoupling.tex]

\begin{longtable}{lllllllllllll}
\caption{Direct happiness–action decoupling index (percentage points).}\label{tab:rq3-direct-decoupling}\\
\toprule
contrast & n\_occurrence\_years & mean\_delta\_happiness\_pp & mean\_delta\_action\_pp & mean\_divergence\_pp & median\_divergence\_pp & ci\_low\_pp & ci\_high\_pp & positive\_divergence\_n & negative\_divergence\_n & wilcoxon\_statistic & wilcoxon\_p\_value & wilcoxon\_q\_value\_bh \\
\midrule
\endfirsthead
\toprule
contrast & n\_occurrence\_years & mean\_delta\_happiness\_pp & mean\_delta\_action\_pp & mean\_divergence\_pp & median\_divergence\_pp & ci\_low\_pp & ci\_high\_pp & positive\_divergence\_n & negative\_divergence\_n & wilcoxon\_statistic & wilcoxon\_p\_value & wilcoxon\_q\_value\_bh \\
\midrule
\endhead
event\_minus\_pre & 19 & 4.944 & -10.75 & 15.69 & 14.41 & 8.604 & 22.78 & 16 & 3 & 12 & 0.000267 & 0.000267 \\
post\_minus\_pre & 19 & 3.392 & -14.03 & 17.42 & 17 & 9.014 & 25.82 & 17 & 2 & 12 & 0.000267 & 0.000267 \\
\bottomrule
\end{longtable}
