# Supplementary material for: AI-inferred expressed well-being and collective-action discourse in climate-change campaigns on X
Source: arXiv:2609.22096 source file (2026-08-11)
Supplement: Supplementary file 7 [file si_table_table_RQ4_campaign_summary.tex]

\begin{longtable}{llllllllllllll}
\caption{Direct happiness–action decoupling by campaign and temporal contrast.}\label{tab:rq4-campaign-summary}\\
\toprule
campaign\_family & contrast & n\_occurrence\_years & mean\_delta\_happiness\_pp & mean\_delta\_action\_pp & mean\_divergence\_pp & median\_divergence\_pp & ci\_low\_pp & ci\_high\_pp & positive\_divergence\_n & negative\_divergence\_n & wilcoxon\_statistic & p\_value & q\_value\_bh \\
\midrule
\endfirsthead
\toprule
campaign\_family & contrast & n\_occurrence\_years & mean\_delta\_happiness\_pp & mean\_delta\_action\_pp & mean\_divergence\_pp & median\_divergence\_pp & ci\_low\_pp & ci\_high\_pp & positive\_divergence\_n & negative\_divergence\_n & wilcoxon\_statistic & p\_value & q\_value\_bh \\
\midrule
\endhead
earth\_day & event\_minus\_pre & 8 & 9.11 & -6.578 & 15.69 & 14.89 & 6.056 & 25.32 & 7 & 1 & 1 & 0.01562 & 0.09375 \\
earth\_hour & event\_minus\_pre & 4 & 0.4693 & -14.31 & 14.78 & 15.11 & -18.08 & 47.64 & 3 & 1 & 1 & 0.25 & 0.25 \\
global\_climate\_action\_day & event\_minus\_pre & 1 & 0.4734 & 8.104 & -7.631 & -7.631 & -- & -- & 0 & 1 & -- & -- & -- \\
world\_environment\_day & event\_minus\_pre & 6 & 3.119 & -17.07 & 20.19 & 21.6 & 5.233 & 35.15 & 6 & 0 & 0 & 0.03125 & 0.09375 \\
earth\_day & post\_minus\_pre & 8 & 5.073 & -5.861 & 10.93 & 9.012 & -1.62 & 23.49 & 7 & 1 & 5 & 0.07812 & 0.1406 \\
earth\_hour & post\_minus\_pre & 4 & 2.842 & -30 & 32.85 & 26.82 & 4.205 & 61.49 & 4 & 0 & 0 & 0.125 & 0.15 \\
global\_climate\_action\_day & post\_minus\_pre & 1 & -0.2195 & -7.88 & 7.661 & 7.661 & -- & -- & 1 & 0 & -- & -- & -- \\
world\_environment\_day & post\_minus\_pre & 6 & 2.12 & -15.29 & 17.41 & 18 & -1.007 & 35.82 & 5 & 1 & 2 & 0.09375 & 0.1406 \\
\bottomrule
\end{longtable}
